# Supplementary material for: On Calibration of LLM-based Guard Models for Reliable Content Moderation
Source: arXiv:2410.10414 source file (2025-02-23)
Supplement: Supplementary file 1 [file app_template.tex]

\begin{figure}[ht]
\begin{AIBox}{Llama-Guard Instruction Template}

\parbox[t]{\textwidth}{{\bf LLaVA-1.5 System Prompt:} \scriptsize\begin{alltt}
A chat between a curious human and an artificial intelligence assistant. The assistant gives helpful, detailed, and polite answers to the human's questions.
\end{alltt}}

\tcbline
\parbox[t]{0.5\textwidth}{\bf \underline{\color{blue}{System Prompt} ${\color{mydarkgreen}\mathcal{S}^{\textrm{V}}}$}} 

\parbox[t]{\textwidth}{{\small \bf Agent Role Prompt} \scriptsize \begin{alltt}
Your environment description contains the following points: <ENVIRONMENT\_DESCRIPTION> \\
Your role description contains the following properties: <ROLE\_DESCRIPTION> \\
Your chat history contains the following records: <CHAT\_HISTORY> \\
Your album contains the following images: <ALBUM\_DESCRIPTION>
\end{alltt}}

\parbox[t]{\textwidth}{{\small \bf Task Prompt} \scriptsize \begin{alltt}
USER: Consider your environment description, role description, and chat history. Please select an image from your album.\\
ASSISTANT: \color{red}{<PLAN>}
\end{alltt}}

\tcbline

\parbox[t]{0.5\textwidth}{\bf \underline{\color{blue}{System Prompt} ${\color{mydarkgreen}\mathcal{S}^{\textrm{Q}}}$}}

\parbox[t]{\textwidth}{{\small \bf Agent Role Prompt} 
\scriptsize \begin{alltt}
Your environment description contains the following points: <ENVIRONMENT\_DESCRIPTION> \\
Your role description contains the following properties: <ROLE\_DESCRIPTION> \\
Your chat history contains the following records: <CHAT\_HISTORY> 
\end{alltt}}

\parbox[t]{\textwidth}{{\small \bf Task Prompt} \scriptsize \begin{alltt}
USER: <image>\\
Consider your environment description, role description and chat history. Please ask a simple question about the image.\\
ASSISTANT: \color{red}{<QUESTION>}
\end{alltt}}

\tcbline

\parbox[h]{0.5\textwidth}{\bf \underline{\color{orange}{System Prompt} ${\color{mydarkgreen}\mathcal{S}^{\textrm{A}}}$}}

\parbox[t]{\textwidth}{{\small \bf Agent Role Prompt} \scriptsize \begin{alltt}
Your environment description contains the following points: <ENVIRONMENT\_DESCRIPTION> \\
Your role description contains the following properties: <ROLE\_DESCRIPTION> \\
Your chat history contains the following records: <CHAT\_HISTORY>
\end{alltt}}

\parbox[t]{\textwidth}{{\small \bf Task Prompt} \scriptsize \begin{alltt}
USER: <image>\\
Consider your environment description, role description and chat history. <QUESTION>\\
ASSISTANT: \color{red}{<ANSWER>}
\end{alltt}}

\end{AIBox}
	\caption{\textbf{System prompts of the multi-agent system for the low diversity scenario.} This shows the LLaVA-1.5 system prompt, our customized system prompts where each of them including the agent role prompt and task prompt for the low diversity scenario.}

	\label{fig:low_prompt}
\end{figure}

% \begin{figure}[ht]
% \begin{AIBox}{Llama-Guard Instruction Template}

% \parbox[t]{\textwidth}{{\bf LLaVA-1.5 System Prompt:} \scriptsize\begin{alltt}
% A chat between a curious human and an artificial intelligence assistant. The assistant gives helpful, detailed, and polite answers to the human's questions.
% \end{alltt}}

% \tcbline
% \parbox[t]{0.5\textwidth}{\bf \underline{\color{blue}{System Prompt} ${\color{mydarkgreen}\mathcal{S}^{\textrm{V}}}$}} 

% \parbox[t]{\textwidth}{{\small \bf Agent Role Prompt} \scriptsize \begin{alltt}
% Your environment description contains the following points: <ENVIRONMENT\_DESCRIPTION> \\
% Your role description contains the following properties: <ROLE\_DESCRIPTION> \\
% Your chat history contains the following records: <CHAT\_HISTORY> \\
% Your album contains the following images: <ALBUM\_DESCRIPTION>
% \end{alltt}}

% \parbox[t]{\textwidth}{{\small \bf Task Prompt} \scriptsize \begin{alltt}
% USER: Consider your environment description, role description, and chat history. Please select an image from your album.\\
% ASSISTANT: \color{red}{<PLAN>}
% \end{alltt}}

% \tcbline

% \parbox[t]{0.5\textwidth}{\bf \underline{\color{blue}{System Prompt} ${\color{mydarkgreen}\mathcal{S}^{\textrm{Q}}}$}}

% \parbox[t]{\textwidth}{{\small \bf Agent Role Prompt} 
% \scriptsize \begin{alltt}
% Your environment description contains the following points: <ENVIRONMENT\_DESCRIPTION> \\
% Your role description contains the following properties: <ROLE\_DESCRIPTION> \\
% Your chat history contains the following records: <CHAT\_HISTORY> 
% \end{alltt}}

% \parbox[t]{\textwidth}{{\small \bf Task Prompt} \scriptsize \begin{alltt}
% USER: <image>\\
% Consider your environment description, role description and chat history. Please ask a simple question about the image.\\
% ASSISTANT: \color{red}{<QUESTION>}
% \end{alltt}}

% \tcbline

% \parbox[h]{0.5\textwidth}{\bf \underline{\color{orange}{System Prompt} ${\color{mydarkgreen}\mathcal{S}^{\textrm{A}}}$}}

% \parbox[t]{\textwidth}{{\small \bf Agent Role Prompt} \scriptsize \begin{alltt}
% Your environment description contains the following points: <ENVIRONMENT\_DESCRIPTION> \\
% Your role description contains the following properties: <ROLE\_DESCRIPTION> \\
% Your chat history contains the following records: <CHAT\_HISTORY>
% \end{alltt}}

% \parbox[t]{\textwidth}{{\small \bf Task Prompt} \scriptsize \begin{alltt}
% USER: <image>\\
% Consider your environment description, role description and chat history. <QUESTION>\\
% ASSISTANT: \color{red}{<ANSWER>}
% \end{alltt}}

% \end{AIBox}
% 	\caption{\textbf{System prompts of the multi-agent system for the low diversity scenario.} This shows the LLaVA-1.5 system prompt, our customized system prompts where each of them including the agent role prompt and task prompt for the low diversity scenario.}

% 	\label{fig:low_prompt}
% \end{figure}
